# Supplementary material for: Stationary Surfaces with Boundaries
Source: arXiv:1912.07103 source file (2021-10-14)
Supplement: Supplementary file 1 [file 09-Appendix.tex]

\section{Appendix}
\subsection{Calculation with Rotational Symmetry}
Locally, we have $\*X:[t_1, t_2]\times \mathbb{S}^{1} \mapsto \mathbb{R}^{3}$
\[M=\*X(t,w) = (t,f(t)w).\]
Computation:
\begin{align*}
F &= (f'^2+1)^{1/2},\\
\*X_{,t} &= (1, f'w),\\
\con &= \frac{\*X_{,t}}{F},\\
\*X_{,i} &= (0, fw_{,i}),\\
\*T &= \frac{\*X_{,i}}{f},\\
\*v &= \frac{1}{F}(-f',w).
\end{align*}
The principal curvatures then are computed accordingly. 
\begin{align*}
h_{tt} &= \frac{f''}{F},\\
h_{ii} &= \frac{-f}{F},\\
H &= \frac{1}{F}(-\frac{1}{f}+\frac{f''}{F^2})=-\frac{1}{fF}+\kappa,\\
|h|^2 &= \frac{1}{f^2F^2}+\kappa^2.
\end{align*}
Recall that the curvature of the curve $(t, f(t))$ is given by
\[ \kappa =\frac{f''}{F^3}.\]

Next we recall
\begin{align*}
g &= F^2 dt^2+ f^2 g_{\mathbb{S}^{1}},\\ 
\Delta &= \frac{1}{F^2}(\partial_t^2 +(\frac{f'}{f}-\frac{F'}{F})\partial_t)+\frac{1}{f^2}\Delta_{\mathbb{S}^{1}}\\
&= \frac{1}{F^2}\partial_t^2+\frac{1}{fF}\partial_t(\frac{f}{F})\partial_t+\frac{1}{f^2}\Delta_{\mathbb{S}^{1}}.
\end{align*} 
When $\partial M$ has the same rotational symmetry as $M$, system (\ref{freecritical}) becomes
\begin{equation*}
\begin{cases}
0 &= 2\Delta H+H(|h|^2-2K) \text{ inside } M,\\
0 &=2h(\con, \con)+(2-c)h(\*T,\*T)  \text{ along } \partial M,\\
0 &= 2\nabla_{\con}H \text{ or } \left\langle{\con,\*v}\right\rangle=0 \text{ along } \partial M.
\end{cases}
\end{equation*}

Next, we restrict to the case $c=4$ for which the functional is conformally invariant. 
\begin{lemma}
System (\ref{freecritical}) becomes
\begin{equation*}
\begin{cases}
0 &= 2\Delta H+H(|h|^2-2K) \text{ inside } M,\\
f'' &=-\frac{F^2}{f} \text{ along } \partial M,\\
f''' &=3\frac{f'F^2}{f^2} \text{ or } \left\langle{\con,\*v}\right\rangle=0 \text{ along } \partial M.
\end{cases}
\end{equation*}	
\end{lemma}
\begin{proof}
	First, for $c=4$, along the boundary,
	\[h(\con, \con)=h(\*T,\*T) \leftrightarrow -\frac{1}{f} =\frac{f''}{F^2}. \] 
	In addition, along the boundary, since $0=\nabla_\con H$, 
	\begin{align*}
	0 &= \partial_t H\\
	 &= \partial_t (-\frac{1}{Ff}+\frac{f''}{F^3})\\
	 &=\frac{F'f+f'F}{F^2f^2}+\frac{f'''F-3F'f''}{F^4}.
	\end{align*}
	Using $-\frac{1}{f} =\frac{f''}{F^2}$ repeatedly yields,
	\begin{align*}
	0 &= \frac{4F'}{fF^2}+\frac{f'}{Ff^2}+\frac{f'''}{F^3},\\
	0 &= 4F'Ff+f'F^2+f^2f'''\\
	&=4ff'f''+f'F^2+f^2f'''\\
	&=-3f'F^2+f^2f'''.  
	\end{align*}
\end{proof}
\begin{remark}
	Since the symmetry of the surface agrees with that of the domain, the system seems to be intrinsic. 
\end{remark}
The Willmore equation is an ODE of fourth order. Indeed, it could be rewritten as a system of first order equations:
\begin{equation}
\label{odesystem}
\begin{cases}
f' &= u,\\
u'&= H(1+u^2)^{3/2}+\frac{1+u^2}{f},\\
H' &=m\frac{\sqrt{1+u^2}}{f},\\
m' &=-(H+\frac{2}{f\sqrt{1+u^2}})^2\frac{Hf\sqrt{1+u^2}}{2}.
\end{cases}
\end{equation}

By standard ODE, the system has a solution as long as $f\neq 0$. Also, if $f'(0)=0$ then we can construct a solution as follows
\begin{align*}
f(t)&=f(-t),\\
u(t)&= -u(-t),\\
H(t)&=H(-t),\\
m(t)&=-m(-t).
\end{align*}
In other words, the solution is symmetrical over each critical point of $f$. 

Another consequence is that, if $H$ is constant then either $f(t)=\frac{1}{b}\cosh(bt), H=0$ or $M$ is circular. 

With respect to this system, the free boundary condition becomes
\begin{align*}
m' &=0  \text{ along } \partial M\\
H' &=0 \text{ or } \left\langle{\con,\*v}\right\rangle=0 \text{ along } \partial M.
\end{align*}

It is then natural to find a symetrical solution. That is equivalent to the following ODE problem.

{\bf ODE Problem:} Given that $f(0)=1, f'(0)=0, f'(t>0)>0$, find conditions on initial data such that system (\ref{odesystem}) has a solution such that there is $T>0$ and $m'(T)=m(T)=0$.

When $h(t)=t$, $H=c$ is constant if and only if
\[f'' f=F^2+ c f F^3.\]
$f$ must be periodic (NEED reference). 
\begin{remark} For a cylinder, $f$ is a positive constant so the mean curvature is a negative constant. 
\end{remark}
\subsection{\textbf{Normal variation of Geodesic and Normal Curvatures}}
If $M$ has a boundary $\partial M=C$ then we will compute how the geodesic and normal curvature of $C\subset M$ evolve. Towards that end, let's recall that, locally, $C$ is a curve with an intrinsic frame $\{\*T, \*N, \*B\}$ satisfying the Serre-Frenet system, for an unit-speed parametrization $s$,
\begin{align*}
\dds \*T &= \kappa\*N,\\
\dds \*N &= -\kappa \*T+\tau \*B,\\
\dds \*B &= -\tau \*N.
\end{align*}
here, $\kappa$ and $\tau$ are the intrinsic curvature and torsion. 

Then, the geodesic curvature $\kappa_g$ and normal curvature $\kappa_n$ depends on how the curve is located in the surface and in $\mathbb{R}^3$. In other words, they can be considered as the curvature of the codimension 2 submanifold $C\subset M\subset \mathbb{R}^3.$ Thus, we consider the extrinsic (to $C$) frame $\{\*T, \*n, \con\}$ with $\con= \*n\times \*T$. The choice of $\*T$ and $\*n$ are such that $\con$ is the outward normal vector to $C\in M$. Then, we have
\begin{align*}
\kappa(s) \*N(s) &= \kappa_n(s)\*n +\kappa_g(s)\con,\\
\kappa_n &= \left\langle{\dds \*T, \*n}\right\rangle=\left\langle{\nabla_\*T \*T, \*n}\right\rangle=h(\*T,\*T),\\
\kappa_g &= \left\langle{\dds \*T, \con}\right\rangle.
\end{align*}

To see how $\kappa_g$ and $\kappa_n$ evolves, we observe that, along a variation $\dds \*r$ might not have unit length. So to be consistent with discussion above, we use a frame to aid calculation. In particular, 
\begin{align*}
\*T(t) &= \frac{d\*r}{ds}/|\frac{d\*r}{ds}|,\\
\con (t) &= \*n(t)\times \*T(t).
\end{align*}

We observe the following preliminary calculation.
\begin{align*}
\Big(\ddt |\frac{d\*r}{ds}|^2\Big)_{\mid {t=0}} &= 2\left\langle{\frac{d\*r}{ds}, \ddt \frac{d\*r}{ds}}\right\rangle\\
&= 2\left\langle{\frac{d\*r}{ds}, \dds \frac{d\*r}{dt}}\right\rangle\\
&= 2\left\langle{\frac{d\*r}{ds}, \dds (u\*n)}\right\rangle\\
&= 2\left\langle{\*T, u_s \*n+u\*n_s}\right\rangle=2\left\langle{\*T, u \*n_s}\right\rangle.
\end{align*}
Thus, 
\begin{equation}
\label{vgn0}
 (\ddt |\frac{d\*r}{ds}|)_{\mid {t=0}} = |\frac{d\*r}{ds}|^{-1} \left\langle{\*T, u \*n_s}\right\rangle=u\left\langle{\*T, \*n_s}\right\rangle.
\end{equation}

\begin{lemma}
	\label{varTandeta}
	Along a normal variation, we have
	\begin{align*}
(\ddt \*T)_{\mid {t=0}} &=u_s \*n-uh(\*T, \con)\con;\\
(\ddt \con)_{\mid {t=0}} &=(\nabla_\con u)\*n+ u h(\*T, \con)\*T;\\
	\end{align*}
\end{lemma}
\begin{proof}
By the definition of $\*T(t)$,
\begin{align*}
(\ddt \*T)_{\mid {t=0}} &=  |\frac{d\*r}{ds}|^{-2}\Big( (\ddt \frac{d\*r}{ds}) |\frac{d\*r}{ds}|-(\ddt  |\frac{d\*r}{ds}|)\frac{d\*r}{ds}\Big)\\
&=|\frac{d\*r}{ds}|^{-2}\Big( |\frac{d\*r}{ds}|(u\*n)_s-|\frac{d\*r}{ds}|^{-1} \left\langle{\*T, u \*n_s}\right\rangle \*T\Big)\\
&= (u\*n)_s-\left\langle{\*T, u \*n_s}\right\rangle \*T. 
\end{align*}
However, 
\begin{align*}
\*n_s &= \nabla_\*T \*n=-h(\*T,\*T)\*T-h(\*T, \con)\con. 
\end{align*}
Therefore, 
\begin{align*}
(\ddt \*T)_{\mid {t=0}} &=u_s \*n-uh(\*T, \con)\con. 
\end{align*}
Similarly, since $\con= \*n\times \*T$, 
\begin{align*}
\ddt \con &= (\ddt \*n)\times \*T+ \*n\times (\ddt \*T),\\
&= (-\nabla u)\times \*T+ \*n\times (u_s \*n-uh(\*T, \con)\con)\\
&=-(\nabla_\con u)(\con\times \*T)-(uh(\*T, \con))\*n\times \con,\\
&=(\nabla_\con u)\*n+ u h(\*T, \con)\*T. 
\end{align*}
\end{proof}

\begin{proposition}
	\label{vargeonor}
Along a proper variation (\ref{eq:normalvar}), the geodesic and normal curvatures evolve by the following equations:
	\begin{align*}
	(\ddt \kappa_g)_{\mid {t=0}} &= u\kappa_n\kappa_g +(\nabla_\con u)\kappa_n-2u_s h(\*T, \con)-u\nabla_\*T h(\*T, \con);\\
	(\ddt \kappa_n)_{\mid {t=0}} &=u_{ss}+u(\kappa_n^2-h(\*T, \con)^2)-\kappa_g (\nabla_\con u)
	\end{align*}
\end{proposition}
\begin{proof}
	Recall, 
	\[ \kappa_g(t)= |\frac{d\*r}{ds}|^{-2}\left\langle{\frac{d^2 \*r}{ds^2}, \con}\right\rangle\]
	Thus, 
	\begin{align}
	(\ddt \kappa_g)_{\mid {t=0}} &= (-2) |\frac{d\*r}{ds}|^{-1} (\ddt |\frac{d\*r}{ds}|)\kappa_g\nonumber \\
	&+|\frac{d\*r}{ds}|^{-2}\left\langle{\ddt \frac{d^2 \*r}{ds^2}, \con}\right\rangle \nonumber\\
		\label{vgn1}
	&+|\frac{d\*r}{ds}|^{-2}\left\langle{\frac{d^2 \*r}{ds^2}, \ddt \con}\right\rangle.
	\end{align}
We will compute each term in the formula above. First, recall that
\begin{align*}
\*n_s &= \nabla_\*T \*n=-h(\*T,\*T)\*T-h(\*T, \con)\con. 
\end{align*} 
Using equation (\ref{vgn0}) yields
\begin{align}
 (-2) (\ddt |\frac{d\*r}{ds}|)\kappa_g &= -2 u\left\langle{\*T, \*n_s}\right\rangle \kappa_g\nonumber \\
\label{vgn2}
 &= 2u h(\*T,\*T)\kappa_g = 2u\kappa_n \kappa_g.
\end{align}
Then, using Lemma \ref{varTandeta}, we have,
\begin{align}
\left\langle{\frac{d^2 \*r}{ds^2}, \ddt \con}\right\rangle &=\left\langle{\frac{d^2 \*r}{ds^2}, (\nabla_\con u)\*n+ u h(\*T, \con)\*T}\right\rangle\nonumber \\
\label{vgn2}
&=(\nabla_\con u)\kappa_n.   
\end{align}

Furthermore, we compute
\begin{align*}
\ddt \frac{d^2 \*r}{ds^2} &= \frac{d^2}{ds^2}(\ddt \*r)=\frac{d^2}{ds^2}(u\*n)\\
&= \dds (u_s \*n+u \*n_s)\\
&=u_{ss}\*n+2u_s \*n_s+u\*n_{ss}.
\end{align*}

Thus,
\begin{align}
\left\langle{\ddt \frac{d^2 \*r}{ds^2}, \con}\right\rangle &= 2u_s\left\langle{\*n_s, \con}\right\rangle+ u\left\langle{\*n_{ss}, \con}\right\rangle \nonumber \\
&= -2u_s h(\*T, \con)-uh(\*T,\*T)\left\langle{\nabla_\*T \*T, \con}\right\rangle-u\nabla_\*T h(\*T, \con)\nonumber \\
\label{vgn3}
&=-2u_s h(\*T, \con)-u\kappa_n\kappa_g-u\nabla_\*T h(\*T, \con)
	\end{align}
Substituting (\ref{vgn0}), (\ref{vgn2}) and (\ref{vgn3}) into (\ref{vgn1}) yields
\begin{align*}
(\ddt \kappa_g)_{\mid {t=0}} &= 2u\kappa_n\kappa_g +(\nabla_\con u)\kappa_n-2u_s h(\*T, \con)-u\kappa_n\kappa_g-u\nabla_\*T h(\*T, \con)\\
&= u\kappa_n\kappa_g +(\nabla_\con u)\kappa_n-2u_s h(\*T, \con)-u\nabla_\*T h(\*T, \con)
\end{align*}

For $\kappa_n$, we recall
	\[ \kappa_n(t)= |\frac{d\*r}{ds}|^{-2}\left\langle{\frac{d^2 \*r}{ds^2}, \*n}\right\rangle\] 
Doing a similar computation yields
\begin{align*}
(\ddt \kappa_n)_{\mid {t=0}} &= (-2)|\frac{d\*r}{ds}|^{-1} (\ddt |\frac{d\*r}{ds}|)\kappa_n
+|\frac{d\*r}{ds}|^{-2}\left\langle{\ddt \frac{d^2 \*r}{ds^2}, \*n}\right\rangle 
+|\frac{d\*r}{ds}|^{-2}\left\langle{\frac{d^2 \*r}{ds^2}, \ddt \*n}\right\rangle\\
&=2u\kappa_n^2+u_{ss}+u\left\langle{\*n_{ss}, \*n}\right\rangle+\left\langle{\frac{d^2 \*r}{ds^2}, -\nabla u}\right\rangle\\
&=2u\kappa_n^2+(\He u)_{ss}-uh(\*T,\*T)^2-uh(\*T, \con)^2\\
&=(\He u)_{ss}+u(\kappa_n^2-h(\*T, \con)^2).
\end{align*}
We observe that
\begin{align*}
(\He u)_{ss} &= u_{ss}-\nabla_{\nabla_\*T \*T}u\\
&= u_{ss}-\kappa_g (\nabla_\con u).
\end{align*}	
The result then follows. 
\end{proof}

Applications:
\begin{theorem}
	A spherical domain $\Omega$ is the critical point of the functional $\int_{\partial \Omega}\kappa^2$ among all boundary-length fixing variations if and only if $\partial \Omega$ is circular. 
\end{theorem}
This might be a known result from the theory of curve-shortening flow. \\

Want to prove: Suppose $\partial \Omega$ is circular and $\Omega$ is a critical point of the above variation problem then $\Omega$ must be either spherical or flat.
